# Supplementary material for: Decision Transformer: Reinforcement Learning via Sequence Modeling
Source: arXiv:2106.01345 source file (2021-06-24)
Supplement: Supplementary file 1 [file experimental_details.tex]

\section{Experimental Details}
